# Supplementary material for: Distributed Embodied Evolution over Networks
Source: arXiv:2003.12848 source file (2020-12-21)
Supplement: Supplementary file 1 [file 6_appendix_imitation.tex]

\section{Additional results on the imitation problem}
\label{app:imitation}

\subsection{$28\times28$ scenario}
We have investigated the effect of $cp$ and $cr$, which affect how frequently crossover occurs, and how many parameters are exchanged respectively. In Figure~\ref{fig:MNISTVectorCompareCR}, we provide the average (across $10$ runs per algorithm) $F_g$ trends of XoverBest and XoverRand for all combinations of $cp \in \{0.2, 0.5, 1.0\}$ and $cr \in \{0.05, 0.2, 0.5\}$. In these experiments, we set $mr = 0.001$. We observe that in general XoverRand performs better than XoverBest. Also, the results indicate a better performance when crossover is performed frequently (higher $cp$) but exchanging small number of components (lower $cr$). In particular, we observe that the best result is achieved using XoverRandCP1CR005, which performs crossover with a randomly selected neighbor exchanging a very small number of components (the expected number of exchanged components per crossover is $0.005\times100 = 5$). 

\subsection{$7\times7$ scenario}
%TODO: actually we did 2 runs
Figure~\ref{fig:comparisonOfCRImitation} shows the average (across $10$ runs per algorithm) $F_g$ trends of a subset of the various versions of the algorithm, with $mr = 0.001$ and selected combinations of $cp \in \{0.2, 0.5, 1.0\}$ and $cr \in \{0.01, 0.1, 0.5\}$. Similarly to the $28\times28$ scenario, HillClimbing and, in general, the versions of the algorithm that do not employ crossover (not shown in the figure), perform worse than those that use it. This shows that even if the optimal parameters of the neighbor agents are quite different (as we have shown in Figure~\ref{fig:compareAgentParameterDistances}), sharing behavior parameters with neighbors helps the optimization process. Also in this scenario, better performance are obtained with high values of $cp$ and lower values of $cr$ (XoverRandCP1CR001).
\begin{figure}[!ht]
\centering
\includegraphics[clip, width=0.8\columnwidth]{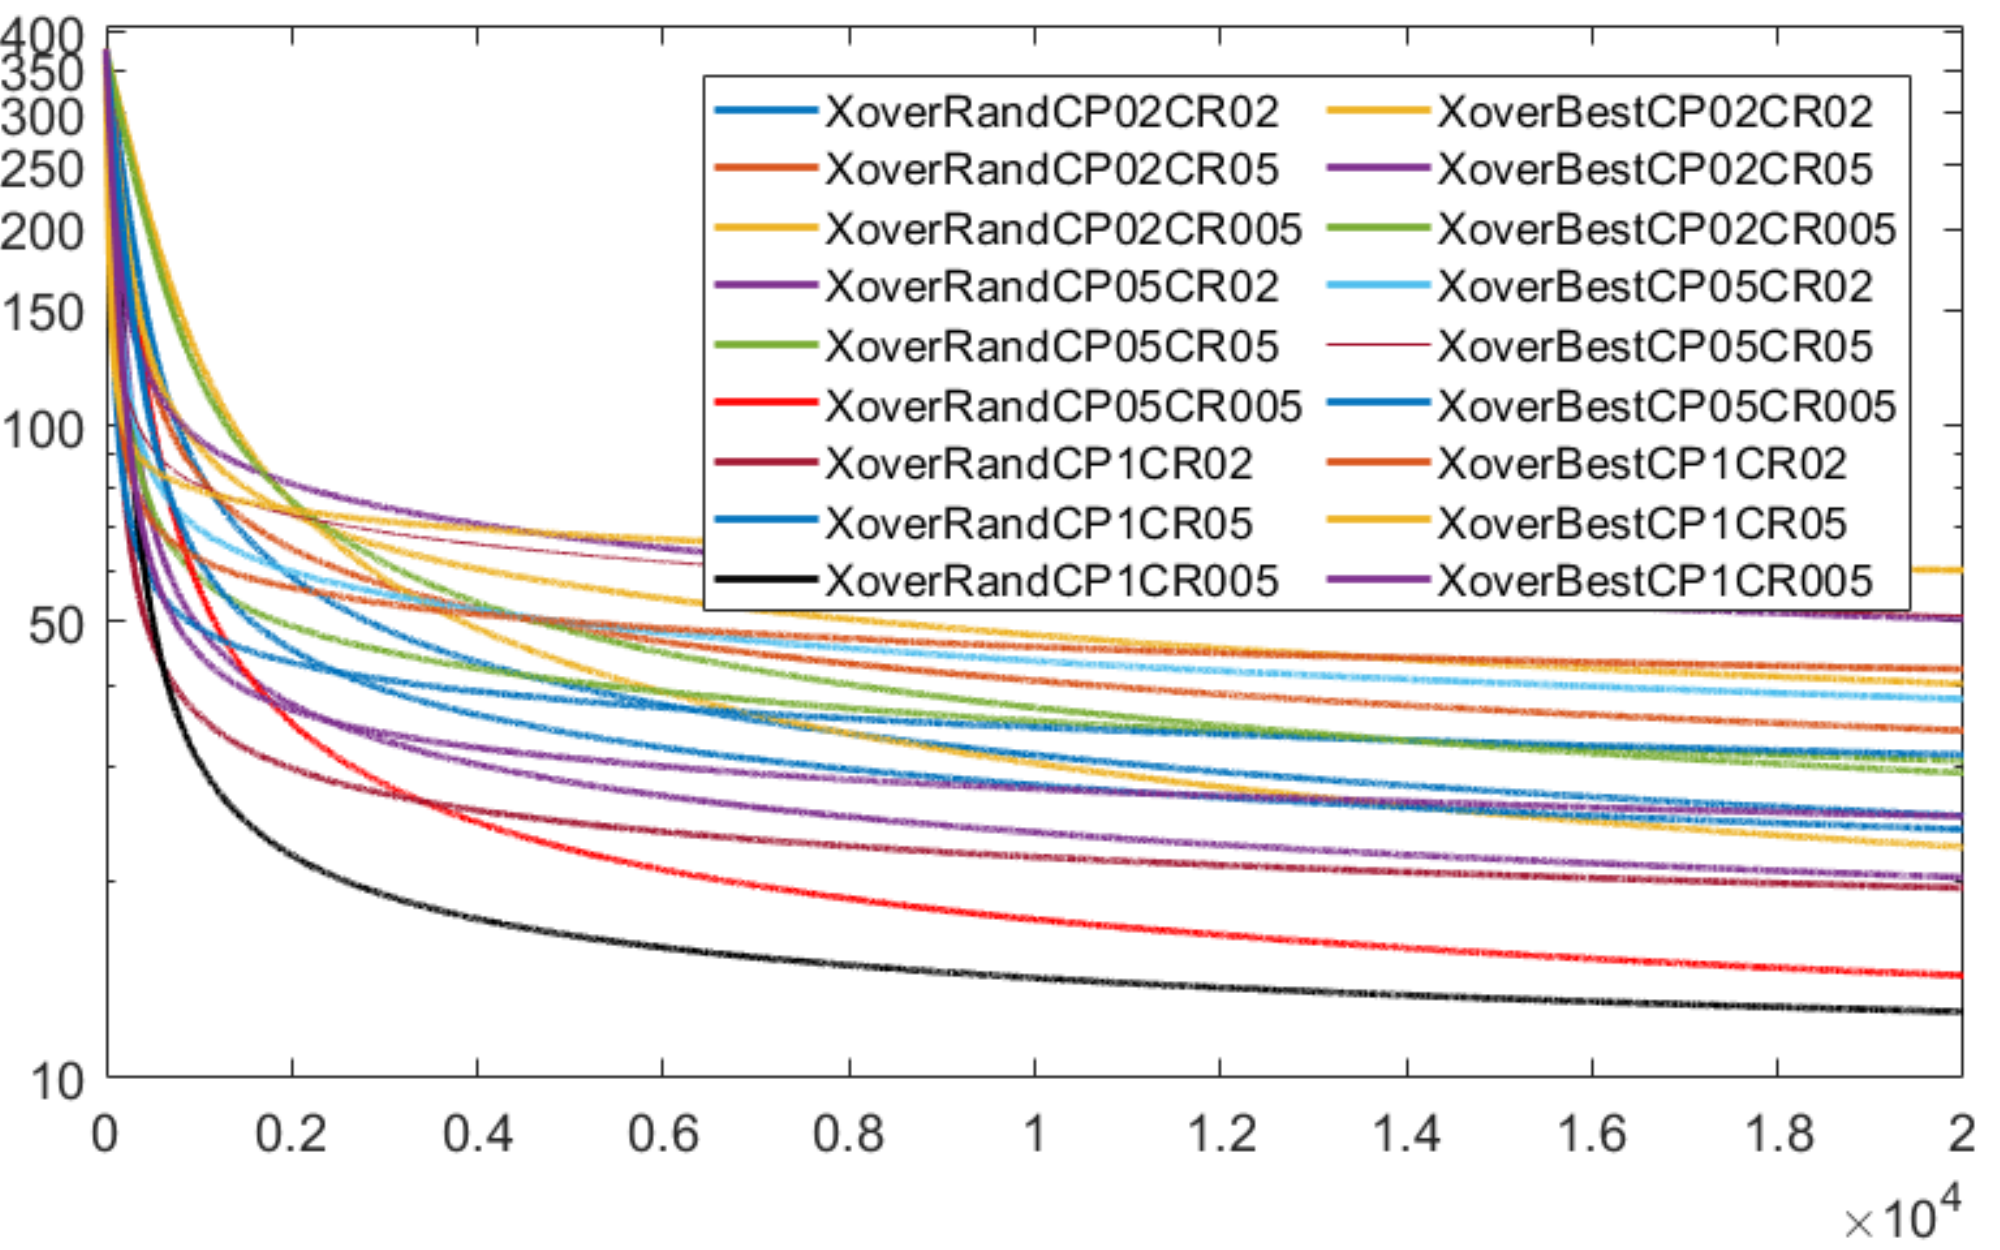}
\caption{Imitation problem ($28\times28$ scenario): Results of different versions of the algorithm with $mr=0.001$ and different values of $cp$ and $cr$.}
\label{fig:MNISTVectorCompareCR}
\end{figure}

\begin{figure}[ht!]
\centering
\includegraphics[clip, width=0.8\columnwidth]{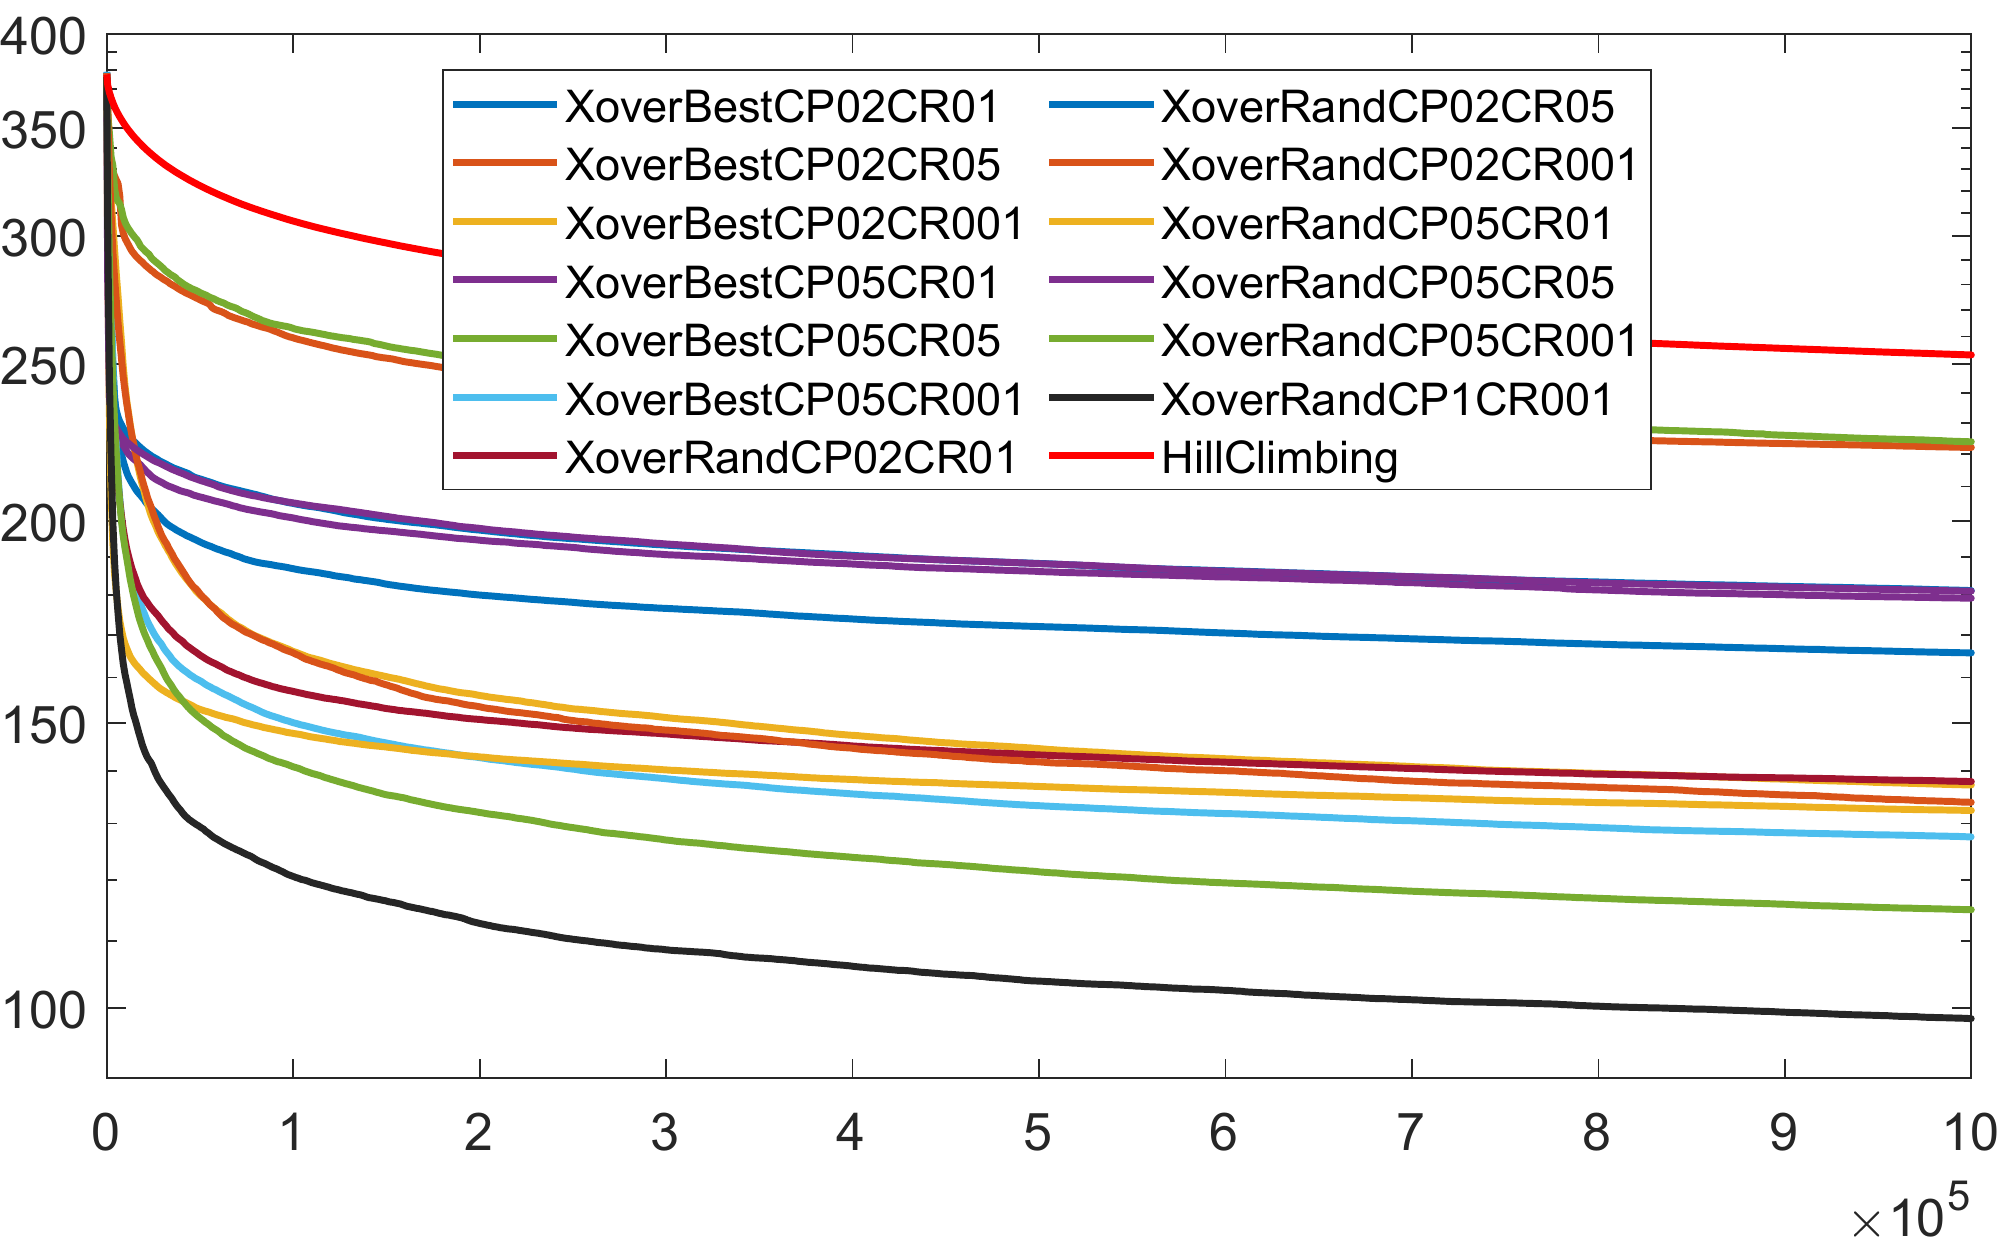}
\caption{Imitation problem ($7\times7$ scenario): Results of different versions of the algorithm with $mr = 0.001$ and different values of $cp$ and $cr$.}
\label{fig:comparisonOfCRImitation}
\end{figure}
